# Supplementary material for: Streaming End-to-End Multilingual Speech Recognition with Joint Language Identification
Source: arXiv:2209.06058 source file (2022-09-13)
Supplement: Supplementary file 1 [file 8_appendix.tex]

\section{Appendix}

\onecolumn
\begin{center}
\begin{longtable}{lccrr}
\caption{Details about the 84 language locales in the second dataset.}\\
\label{tab:example}
\endfirsthead
\endhead
\toprule
\textbf{LID} & \textbf{Language} & \textbf{Region} & \textbf{Utterance Counts(K)} & \textbf{Durations (hours)} \\
\midrule
af-ZA & Afrikaans & South Africa & 1,914 & 2,067.9 \\
am-ET & Amharic & Ethiopia & 542 & 924.7 \\
ar-EG & Arabic & Egypt & 5435 & 6,634.2 \\
ar-X-GULF & Arabic & Arabia & 5,193 & 6,136.6 \\
ar-X-LEVANT & Arabic & Levant & 10,743 & 12,634.1 \\
ar-X-MAGHREBI & Arabic & Maghrebi & 6,204 & 6,102.4 \\
az-AZ & Azerbaijani & Azerbaijan & 487 & 553.2 \\
be-BY & Belarusian & Belarus & 733 & 1,072.6 \\
bg-BG & Bulgarian & Bulgaria & 7,828 & 7,946.8 \\
bn-BD & Bangla & Bangladesh & 4,240 & 4,870.5 \\
ca-ES & Catalan & Spain & 1,127 & 1,231.7 \\
cmn-HANS-CN & Simplified Chinese & Mainland China & 163 & 167.9 \\
%cmn-HANS-X-DALU & Simplified Chinese & China (Mainland) & 5416 & 3644.8 \\
cmn-HANT-TW & Traditional Chinese & Taiwan & 13,408 & 14,396.0 \\
cs-CZ & Czech & Czechia & 6,420 & 6,272.4 \\
da-DK & Danish & Denmark & 2,914 & 2,660.2 \\
de-DE & German & Germany & 19,713 & 21,002.3 \\
el-GR & Greek & Greece & 4,972 & 4,877.8 \\
en-AU & English & Australia & 14,977 & 15,344.3 \\
en-GB & English & United Kingdom & 11,887 & 11,847.9 \\
en-IN & English & India & 16526 & 19,922.4 \\
en-PH & English & Philippines & 3,723 & 4,171.8 \\
en-US & English & United States & 43,063 & 49,483.0 \\
en-X-UNIFIED & English & Ghana, Kenya, South Africa, etc & 10,336 & 12,546.3 \\
es-ES & Spanish & Spain & 29,576 & 36,048.0 \\
es-US & Spanish & United States & 42,722 & 53,182.1 \\
et-EE & Estonian & Estonia & 1,126 & 997.2 \\
eu-ES & Basque & Spain & 583 & 669.6 \\
fa-IR & Persian & Iran & 2566 & 2,760.6 \\
fi-FI & Finnish & Finland & 4478 & 3,958.6 \\
fil-PH & Filipino & Philippines & 1,809 & 1,872.3 \\
fr-CA & French & Canada & 10810 & 10,002.3 \\
fr-FR & French & France & 40495 & 40,280.2 \\
gl-ES & Galician & Spain & 446 & 464.9 \\
gu-IN & Gujarati & India & 3498 & 4,116.6 \\
he-IL & Hebrew & Israel & 6332 & 6,342.7 \\
hi-IN & Hindi & India & 18230 & 23,088.9 \\
hu-HU & Hungarian & Hungary & 5,966 & 5,725.5 \\
hy-AM & Armenian & Armenia & 967 & 1,303.0 \\
id-ID & Indonesian & Indonesia & 23,140 & 30,576.0 \\
is-IS & Icelandic & Iceland & 885 & 836.1 \\
it-IT & Italian & Italy & 19,691 & 23,612.4 \\
ja-JP & Japanese & Japan & 27,632 & 28,391.0 \\
jv-ID & Javanese & Indonesia & 419 & 402.6 \\
ka-GE & Georgian & Georgia & 821 & 643.5 \\
kk-KZ & Kazakh & Kazakhstan & 168 & 326.3 \\
km-KH & Khmer & Cambodia & 998 & 734.8 \\
kn-IN & Kannada & India & 1013 & 1,304.1 \\
ko-KR & Korean & South Korea & 22,232 & 26,372.5 \\
lo-LA & Lao & Laos & 883 & 584.1 \\
lt-LT & Lithuanian & Lithuania & 2,115 & 2,271.3 \\
lv-LV & Latvian & Latvia & 1222 & 1,017.1 \\
mk-MK & Macedonian & North Macedonia & 934 & 1,152.4 \\
ml-IN & Malayalam & India & 882 & 1,380.0 \\
mn-MN & Mongolian & Mongolia & 848 & 1,075.1 \\
mr-IN & Marathi & India & 8,603 & 9,793.4 \\
ms-MY & Malay & Malaysia & 5,989 & 6,920.5 \\
my-MM & Burmese & Myanmar (Burma) & 905 & 696.9 \\
nb-NO & Norwegian & Norway & 4,343 & 4,051.6 \\
ne-NP & Nepali & Nepal & 972 & 1,480.7 \\
nl-NL & Dutch & Netherlands & 8,618 & 8,475.3 \\
pa-GURU-IN & Punjabi & India & 1,586 & 1,621.3 \\
pl-PL & Polish & Poland & 14218 & 18,139.9 \\
pt-BR & Portuguese & Brazil & 14,558 & 17,768.9 \\
pt-PT & Portuguese & Portugal & 4,740 & 5,585.9 \\
ro-RO & Romanian & Romania & 15,767 & 19,972.2 \\
ru-RU & Russian & Russia & 27,303 & 34,658.1 \\
si-LK & Sinhala & Sri Lanka & 1,212 & 1,166.3 \\
sk-SK & Slovak & Slovakia & 3,641 & 3,549.4 \\
sl-SI & Slovenian & Slovenia & 1,321 & 1,123.4 \\
sq-AL & Albanian & Albania & 746 & 747.1 \\
sr-RS & Serbian & Serbia & 5,271 & 5,581.3 \\
su-ID & Sundanese & Indonesia & 409 & 466.7 \\
sv-SE & Swedish & Sweden & 6,659 & 6,474.9 \\
sw & Swahili & Tanzania, etc. & 1,638 & 1,344.2 \\
ta-IN & Tamil & India & 3,558 & 3,948.9 \\
te-IN & Telugu & India & 2,438 & 2,858.2 \\
th-TH & Thai & Thailand & 8,528 & 8,904.5 \\
tr-TR & Turkish & Turkey & 15,774 & 18,732.0 \\
uk-UA & Ukrainian & Ukraine & 11,957 & 15,648.3 \\
ur-PK & Urdu & Pakistan & 673 & 869.6 \\
uz-UZ & Uzbek & Uzbekistan & 593 & 897.7 \\
vi-VN & Vietnamese & Vietnam & 10,263 & 10,622.0 \\
yue-HANT-HK & Cantonese & Hong Kong & 4,940 & 4,644.8 \\
zu-ZA & Zulu & South Africa & 669 & 917.6 \\
\bottomrule
\end{longtable}
\end{center}
